# Supplementary material for: Convexifying Market Clearing of SoC-Dependent Bids from Merchant Storage Participants
Source: arXiv:2209.02107 source file (2023-02-01)
Supplement: Supplementary file 1 [file Appendix_v6.tex]

\subsection{Proof of Lemma~\ref{lemma:bidSpread}}
Proof: We prove Lemma~\ref{lemma:bidSpread} by contradiction with the subgradient optimality condition \cite{KKT16CMU} without assuming convexity and differentiability.

The Lagrangian function of  (\ref{eq:NONCVX}) is
\beq
\begin{array}{clc}
&    {\cal L}&= \sum_{t=1}^T\bigg(\varphi(\gbf^{\mbox{\tiny G}}[t],\gbf^{\mbox{\tiny C}}[t], \gbf^{\mbox{\tiny D}}[t])  +\pmb{\mubf}[t]^\intercal( \Sbf (\gbf^{\mbox{\tiny G}}[t]+\gbf^{\mbox{\tiny D}}[t]-{\gbf}^{\mbox{\tiny C}}[t]\\
&&-\dbf[t])- \qbf)+\lambda_{t}({\bf 1}^\intercal \dbf[t]-( {\bf 1}^\intercal (\gbf^{\mbox{\tiny G}}[t]+\gbf^{\mbox{\tiny D}}]t]-\gbf^{\mbox{\tiny C}}[t]))) \\
&&+\sum_i \big(\phi_{it}(e_{i(t+1)}-(e_{it}+g^{\mbox{\tiny C}}_{it}\eta^{\mbox{\tiny C}}-g^{\mbox{\tiny D}}_{it}/\eta^{\mbox{\tiny D}}))\\
&& +\underline{\rho}^{\mbox{\tiny G}}_i(-g^{\mbox{\tiny G}}_{it})+\bar{\rho}^{\mbox{\tiny G}}_i(g^{\mbox{\tiny G}}_{it} - \bar{g^{\mbox{\tiny G}}_i},)+...\big)\bigg).
\end{array}
\eeq

The stationary condition gives that \footnote{For simplicity, storage index $i$ is omitted here.} 
\[
\begin{cases} 
0 \in \frac{\partial}{\partial g^{\mbox{\tiny C}}_{it}}   {\cal L}(g^{\mbox{\tiny C}*}_{it}, g^{\mbox{\tiny D}*}_{it};e^*_{it},...) ,& \\
0 \in \frac{\partial}{\partial g^{\mbox{\tiny D}}_{it}}  {\cal L}(g^{\mbox{\tiny C}*}_{it}, g^{\mbox{\tiny D}*}_{it};e^*_{it},...) , & 
\end{cases}
\]

\textcolor{red}{exist dual variables from the normal cone of cooresponding constraints, and we have zero equal to that.}

Assume there exists an optimal solution with simultaneous charging and discharging behavior, \ie $g^{\mbox{\tiny C}*}_{it}>0, g^{\mbox{\tiny D}*}_{it}>0$. Known that  (\ref{eq:NONCVX}) has a subdifferentiable objective function and a (closed) convex feasible set. From the  KKT conditions of  (\ref{eq:NONCVX}) we know \footnote{For simplicity, storage index $i$ is omitted here.}  that there exist $ \kappa^{\mbox{\tiny C}} \in \frac{\partial}{\partial g^{\mbox{\tiny C}}_{it}}  f_i(\xbf^*) ,  \kappa^{\mbox{\tiny D}} \in \frac{\partial}{\partial g^{\mbox{\tiny D}}_{it}}  f_i(\xbf^*) $, $\lambda^* \in {\cal N}_{{\bf 1}^\intercal (\gbf^{\mbox{\tiny G}}[t]+\gbf^{\mbox{\tiny D}}]t]-\gbf^{\mbox{\tiny C}}[t])={\bf 1}^\intercal \dbf[t]}(\xbf^*)$, such that
\[
\begin{cases} 
 \kappa^{\mbox{\tiny C}} +\lambda^*_t-\phi^*_t\eta^{\mbox{\tiny C}}-\underline{\rho}^{\mbox{\tiny C}*}+\bar{\rho}^{\mbox{\tiny C}*}=0,& \\
 \kappa^{\mbox{\tiny D}}-\lambda^*_t+\phi_t^*/\eta^{\mbox{\tiny D}}-\underline{\rho}^{\mbox{\tiny D}*}+\bar{\rho}^{\mbox{\tiny D}*}=0, & 
\end{cases}
\]
\[\Rightarrow  \frac{1}{\eta^{\mbox{\tiny C}}} \kappa^{\mbox{\tiny C}} +\kappa^{\mbox{\tiny D}}+\lambda^*_t(\frac{1}{\eta^{\mbox{\tiny C}}}-\eta^{\mbox{\tiny D}})+\frac{\bar{\rho}^{\mbox{\tiny C}*}}{\eta^{\mbox{\tiny C}}}+\bar{\rho}^{\mbox{\tiny C}*}\eta^{\mbox{\tiny D}}=0
\]
%\[\Rightarrow 0 \in {\cal C}(g^{\mbox{\tiny C}*}_{it}, g^{\mbox{\tiny D}*}_{it};e^*_{it})+\lambda^*_t(\frac{1}{\eta^{\mbox{\tiny C}}}-\eta^{\mbox{\tiny D}})+\frac{\bar{\rho}^{\mbox{\tiny C}*}}{\eta^{\mbox{\tiny C}}}+\bar{\rho}^{\mbox{\tiny C}*}\eta^{\mbox{\tiny D}},\]
where $\underline{\rho}^{\mbox{\tiny C}*}=0, \underline{\rho}^{\mbox{\tiny D}*}=0,\bar{\rho}^{\mbox{\tiny C}*}\geq 0, \bar{\rho}^{\mbox{\tiny D}*}\geq 0, \frac{1}{\eta^{\mbox{\tiny C}}}\geq 1 \geq \eta^{\mbox{\tiny D}}$, and 
%\[{\cal C}(g^{\mbox{\tiny C}*}_{it}, g^{\mbox{\tiny D}*}_{it};e^*_{it}):=\frac{-1}{\eta^{\mbox{\tiny C}}}\frac{\partial}{\partial g^{\mbox{\tiny C}}_{it}}  f_i(g^{\mbox{\tiny C}}_{it}, g^{\mbox{\tiny D}}_{it};e_{it}) +\eta^{\mbox{\tiny D}}\frac{\partial}{\partial g^{\mbox{\tiny D}}_{it}}  f_i(g^{\mbox{\tiny C}}_{it}, g^{\mbox{\tiny D}}_{it};e_{it}).\] 

Subgradient of storage cost function has  (Similarly for $\frac{\partial}{\partial g^{\mbox{\tiny D}}_{it}}  f_i(g^{\mbox{\tiny C}}_{it}, g^{\mbox{\tiny D}}_{it};e_{it})$)
\[\frac{\partial}{\partial g^{\mbox{\tiny C}}_{it}}  f_i(g^{\mbox{\tiny C}}_{it}, g^{\mbox{\tiny D}}_{it};e_{it}) =\begin{cases} -c^{\mbox{\tiny C}}_{k}, &  g^{\mbox{\tiny C}}_{it}\in(E_{ik}, E_{i(k+1)})\\
[-c^{\mbox{\tiny C}}_{k+1}, -c^{\mbox{\tiny C}}_{k}], & g^{\mbox{\tiny C}}_{it}=E_{i(k+1)} .\end{cases}\]

Under Assumption~\ref{assume:single} , we have $ \frac{1}{\eta^{\mbox{\tiny C}}} \kappa^{\mbox{\tiny C}} +\kappa^{\mbox{\tiny D}}> 0$.

This contradict to the condition that $\lambda_t^*\geq 0, \forall t$. 

\subsection{Proof of Theorem~\ref{thm:Eq}}
Proof:  we prove Theorem~\ref{thm:Eq} for all $T$ by induction.

1) Let $T=1$, total cost of storage can be computed by (\ref{eq:StageCost}), which is (\ref{eq:ES_cost}) with  $T=1$. 

2) Assume Theorem~\ref{thm:Eq} is true at time $T$, and here we proof that Theorem~\ref{thm:Eq} is true at $T+1$.  Let $r$ being the index for SoC-partitioned set that has $e_{\mbox{\tiny T+2}}\in \Ec_{r}$.

i. \underline{When $r=n$}, the total cost of storage at time $T+1$, i.e. $F(\gbf^{\mbox{\tiny C}}, \gbf^{\mbox{\tiny D}};s)=\sum_{t=1}^{T+1}f(g^{\mbox{\tiny C}}_{t}, g^{\mbox{\tiny D}}_{t};e_{t})$ equals to
\beq
\begin{array}{lrl}
\sum_{t=1}^{T}f(g^{\mbox{\tiny C}}_{t}, g^{\mbox{\tiny D}}_{t};e_{t})-c^{\mbox{\tiny C}}_{n}g^{\mbox{\tiny C}}_{\mbox{\tiny T+1}}+c^{\mbox{\tiny D}}_{n}g^{\mbox{\tiny D}}_{\mbox{\tiny T+1}}\\
~~~~=-c^{\mbox{\tiny C}}_{r}(\sum_{t=1}^{ T+1}g^{\mbox{\tiny C}}_t)+c^{\mbox{\tiny D}}_{r}(\sum_{t=1}^{ T+1}g^{\mbox{\tiny D}}_t)\\
~~~~~~~~+\begin{cases}
\sum_{k=m}^{r-1}\frac{-\Delta c^{\mbox{\tiny C}}_{k}}{\eta^{\mbox{\tiny C}}}(E_{k+1}-s), & r>m  \\
0, & r=m  \\
\sum_{k=r+1}^{m}\eta^{\mbox{\tiny D}}\Delta c^{\mbox{\tiny D}}_{k-1}(E_{k}-s), & r<m
\end{cases},\nn
\end{array}
\eeq
which is equivalent to (\ref{eq:ES_cost}) in Theorem~\ref{thm:Eq}.

ii. \underline{When $r>n$}, we have $g^{\mbox{\tiny C}}_{\mbox{\tiny T+1}}>0, g^{\mbox{\tiny D}}_{\mbox{\tiny T+1}}=0$ from Lemma~\ref{lemma:bidSpread}. Since $f^{\mbox{\tiny C}}(e_{\mbox{\tiny T+1}}, g_{\mbox{\tiny T+1}}^{\mbox{\tiny C}})=  g^{\mbox{\tiny C}}_tc^{\mbox{\tiny C}}_{r} +\sum_{k=n}^{r-1}\frac{\Delta c^{\mbox{\tiny C}}_{k}}{\eta^{\mbox{\tiny C}}}(E_{k+1}-e_t).$ and $e_{t+1}=e_1+\sum_{t'=1}^{t}(g^{\mbox{\tiny C}}_{t'}\eta^{\mbox{\tiny C}}-g^{\mbox{\tiny D}}_{t'}/\eta^{\mbox{\tiny D}}), \forall t$, the total cost of storage at time $T+1$ when $n>m$ is given by
\beq
\begin{array}{lcl}
&F(\gbf^{\mbox{\tiny C}}, \gbf^{\mbox{\tiny D}};s)=\sum_{t=1}^{T}f(g^{\mbox{\tiny C}}_{t}, g^{\mbox{\tiny D}}_{t};e_{t})-f^{\mbox{\tiny C}}(e_{\mbox{\tiny T+1}}, g_{\mbox{\tiny T+1}}^{\mbox{\tiny C}}),\\
&~~~~~~~~=\sum_{t=1}^{T+1}(c^{\mbox{\tiny D}}_{r}g^{\mbox{\tiny D}}_t-c^{\mbox{\tiny C}}_{r}g^{\mbox{\tiny C}}_t)-\sum_{k=m}^{r-1}\frac{\Delta c^{\mbox{\tiny C}}_{k}}{\eta^{\mbox{\tiny C}}}(E_{k+1}-s),\nn
\end{array}
\eeq%$f^{\mbox{\tiny C}}(e_{t}, g_{t}^{\mbox{\tiny C}})$ for equation (\ref{eq:StageCost}), we know 
with $\frac{c^{\mbox{\tiny C}}_k-c^{\mbox{\tiny C}}_{k-1}}{c^{\mbox{\tiny D}}_k-c^{\mbox{\tiny D}}_{k-1}}=\eta^{\mbox{\tiny C}}\eta^{\mbox{\tiny D}}, \forall k$. Similarly, when $n=m$ and $n<m$, we can show total cost of storage at time $T+1$ is 
\beq
\begin{array}{lrl}
F(\gbf^{\mbox{\tiny C}}, \gbf^{\mbox{\tiny D}};s)
=\sum_{t=1}^{T+1}(c^{\mbox{\tiny D}}_{r}g^{\mbox{\tiny D}}_t-c^{\mbox{\tiny C}}_{r}g^{\mbox{\tiny C}}_t)\\
~~~~~~~~~~~~~~~~+\begin{cases}
\sum_{k=m}^{r-1}\frac{-\Delta c^{\mbox{\tiny C}}_{k}}{\eta^{\mbox{\tiny C}}}(E_{k+1}-s), & r>m  \\
0, & r=m  \\
\sum_{k=r+1}^{m}\eta^{\mbox{\tiny D}}\Delta c^{\mbox{\tiny D}}_{k-1}(E_{k}-s), & r<m
\end{cases}.\nn
\end{array}
\eeq

iii.\underline{When $r<n$}, similar proofs work.  So Theorem~\ref{thm:Eq}  is true at time $T+1$. From Assumption~\ref{assume:single}, we know (\ref{eq:ES_cost}) is convex.
% \footnote{Note that, in above equations and proofs, the case of 1 storage is considered, and similar proof works for multiple storage.}.
